# Supplementary material for: Extension of the CIPSI-Driven CC($P$;$Q$) Approach to Excited Electronic States
Source: arXiv:2601.11856 ancillary file (2026-02-12)
Supplement: Supplementary file 1 [file supplementary_data.pdf]

# Supplementary Data for
# Extension of the CIPSI-Driven CC($P$;$Q$) Approach to Excited Electronic States

Swati S. Priyadarsini[a], Karthik Gururangan[a], Piotr Piecuch[a,b,*]

[a]*Department of Chemistry, Michigan State University, East Lansing, Michigan 48824, USA*
[b]*Department of Physics and Astronomy, Michigan State University, East Lansing, Michigan 48824, USA*

This Supplementary Data document compares the results of the CIPSI-driven CC($P$), EOMCC($P$), and CC($P$;$Q$) calculations for the ground- and excited-state PES cuts of the water molecule, as described by the TZ basis set of Ref. [S1], corresponding to the $H_2O \rightarrow H + OH$ dissociation with the parent CCSDT/EOMCCSDT data.

## References

(S1) X. Li, J. Paldus, Performance of multireference and equation-of-motion coupled-cluster methods for potential energy surfaces of low-lying excited states: Symmetric and asymmetric dissociation of water, J. Chem. Phys. 133 (2010) 024102. doi:10.1063/1.3451074.

*Corresponding author
*Email address:* piecuch@chemistry.msu.edu (Piotr Piecuch)

**Table S1**

The total electronic energies, reported as errors relative to CCSDT in millihartree, obtained with the CIPSI-driven CC($P$) and CC($P$;$Q$) approaches for the X $^1$A′ state of the water molecule, as described by the TZ basis set of Ref. [S1], along the O–H bond-breaking coordinate, $R_{\mathrm{OH}}$, in bohr. The lowest-energy orbital correlating with the 1s shell of oxygen was kept frozen in post-RHF steps.

| $R_{\mathrm{OH}}$ | $N_{\mathrm{det(in)}} = 1$[a] | | $N_{\mathrm{det(in)}} = 1{,}000$ | | $N_{\mathrm{det(in)}} = 5{,}000$ | | $N_{\mathrm{det(in)}} = 10{,}000$ | | $N_{\mathrm{det(in)}} = 20{,}000$ | |
|---|---|---|---|---|---|---|---|---|---|---|
| | %T=0.0[b] | | %T=0.0–0.6[b] | | %T=3.1–9.3[b] | | %T=8.1–15.6[b] | | %T=16.7–29.1[b] | |
| | $P$[c] | ($P$;$Q$)[d] | $P$[c] | ($P$;$Q$)[d] | $P$[c] | ($P$;$Q$)[d] | $P$[c] | ($P$;$Q$)[d] | $P$[c] | ($P$;$Q$)[d] |
| 1.3 | 2.771 | −0.226 | 2.712 | −0.214 | 1.486 | −0.065 | 0.867 | −0.026 | 0.432 | −0.009 |
| 1.6 | 3.063 | −0.269 | 2.539 | −0.176 | 1.241 | −0.049 | 0.792 | −0.023 | 0.372 | −0.006 |
| 1.809[e] | 3.307 | −0.298 | 2.767 | −0.201 | 1.431 | −0.056 | 0.539 | −0.013 | 0.167 | −0.002 |
| 2.0 | 3.562 | −0.325 | 3.351 | −0.283 | 1.540 | −0.060 | 1.083 | −0.035 | 0.563 | −0.016 |
| 2.4 | 4.230 | −0.398 | 4.230 | −0.398 | 1.849 | −0.082 | 1.087 | −0.037 | 0.431 | −0.010 |
| 2.8 | 5.150 | −0.500 | 4.107 | −0.357 | 2.008 | −0.107 | 1.183 | −0.048 | 0.533 | −0.015 |
| 3.2 | 6.389 | −0.613 | 4.282 | −0.355 | 1.444 | −0.083 | 0.695 | −0.024 | 0.265 | −0.007 |
| 3.6 | 7.929 | −0.724 | 3.376 | −0.265 | 1.473 | −0.077 | 0.990 | −0.044 | 0.495 | −0.017 |
| 4.0 | 9.622 | −0.828 | 3.228 | −0.243 | 1.369 | −0.069 | 0.867 | −0.035 | 0.440 | −0.014 |
| 4.2 | 10.448 | −0.875 | 3.203 | −0.230 | 1.322 | −0.065 | 0.819 | −0.031 | 0.432 | −0.015 |
| 4.4 | 11.224 | −0.918 | 2.971 | −0.197 | 0.817 | −0.032 | 0.806 | −0.030 | 0.389 | −0.012 |

[a] The CC($P$) and CC($P$;$Q$) results for the X $^1$A′ state at $N_{\mathrm{det(in)}} = 1$ are equivalent to those obtained with CCSD and CR-CC(2,3), respectively.

[b] The %T for a given $N_{\mathrm{det(in)}}$ is the percentage ($N_{\mathrm{det(in)}} = 1$) or the range of percentages ($N_{\mathrm{det(in)}} = 1{,}000$–$20{,}000$) of the $S_z = 0$ triply excited determinants captured by the CIPSI runs for the X $^1$A′ ground state at the various geometries of $H_2O$ used to construct the ground- and excited-state potentials considered in the present study.

[c] Errors, in millihartree, characterizing the CC($P$) energies relative to the corresponding CCSDT data, which are −76.015602, −76.148832, −76.168316, −76.163964, −76.130217, −76.091972, −76.060470, −76.037848, −76.023323, −76.018463, and −76.014832 hartree for $R_{\mathrm{OH}}$ = 1.3, 1.6, 1.809, 2.0, 2.4, 2.8, 3.2, 3.6, 4.0, 4.2, and 4.4, respectively.

[d] Errors, in millihartree, in the CC($P$;$Q$) energies relative to the corresponding CCSDT data given in footnote ‘c’.

[e] The equilibrium value of the O–H bond length in the ground electronic state of water, as obtained in Ref. [S1] using the CCSD/cc-pVTZ method.

**Table S2**

The total electronic energies, reported as errors relative to EOMCCSDT in millihartree, obtained with the CIPSI-driven EOMCC($P$) and CC($P$;$Q$) approaches for the 1 $^1$A″ state of the water molecule, as described by the TZ basis set of Ref. [S1], along the O–H bond-breaking coordinate, $R_{OH}$, in bohr. The lowest-energy orbital correlating with the 1s shell of oxygen was kept frozen in post-RHF steps.

| $R_{OH}$ | $N_{det(in)} = 1$[a] | | $N_{det(in)} = 1,000$ | | $N_{det(in)} = 5,000$ | | $N_{det(in)} = 10,000$ | | $N_{det(in)} = 20,000$ | |
|---|---|---|---|---|---|---|---|---|---|---|
| | %T=0.0[b] | | %T=2.2–4.3[b] | | %T=9.7–15.9[b] | | %T=13.7–23.7[b] | | %T=19.5–34.7[b] | |
| | $P$[c] | ($P$;$Q$)[d] | $P$[c] | ($P$;$Q$)[d] | $P$[c] | ($P$;$Q$)[d] | $P$[c] | ($P$;$Q$)[d] | $P$[c] | ($P$;$Q$)[d] |
| 1.3 | −0.081 | 0.917 | −0.081 | 1.034 | 1.306 | 0.711 | 0.885 | 0.422 | 0.398 | 0.270 |
| 1.6 | 0.049 | 1.125 | 3.034 | 0.992 | 1.415 | 0.669 | 0.845 | 0.475 | 0.430 | 0.270 |
| 1.809[e] | 0.301 | 1.145 | 0.128 | 1.046 | −0.384 | 0.709 | −0.749 | 0.416 | −0.968 | 0.213 |
| 2.0 | 1.015 | 1.005 | 3.180 | 1.084 | 1.510 | 0.688 | 0.939 | 0.552 | 0.478 | 0.306 |
| 2.4 | 4.320 | 0.505 | 3.361 | 0.552 | 1.583 | 0.633 | 0.707 | 0.379 | 0.313 | 0.197 |
| 2.8 | 7.904 | −0.067 | 3.408 | 0.531 | 1.571 | 0.693 | 0.859 | 0.477 | 0.389 | 0.211 |
| 3.2 | 10.917 | −0.875 | 4.354 | 0.528 | 1.208 | 0.603 | 0.616 | 0.311 | 0.298 | 0.147 |
| 3.6 | 13.263 | −1.810 | 3.319 | 0.816 | 1.336 | 0.724 | 0.956 | 0.502 | 0.448 | 0.313 |
| 4.0 | 14.933 | −2.700 | 2.909 | 0.902 | 1.270 | 0.758 | 0.810 | 0.535 | 0.510 | 0.360 |
| 4.2 | 15.537 | −3.095 | 4.129 | 0.930 | 1.100 | 0.638 | 0.789 | 0.547 | 0.372 | 0.249 |
| 4.4 | 16.012 | −3.448 | 4.451 | 0.969 | 0.963 | 0.436 | 0.705 | 0.428 | 0.339 | 0.207 |

[a] The EOMCC($P$) and CC($P$;$Q$) results for the 1 $^1$A″ state at $N_{det(in)} = 1$ are equivalent to those obtained with EOMCCSD and CR-EOMCC(2,3), respectively.

[b] The %T for a given $N_{det(in)}$ is the percentage ($N_{det(in)} = 1$) or the range of percentages ($N_{det(in)} = 1,000$–$20,000$) of the $S_z = 0$ triply excited determinants captured by the CIPSI runs for the 1 $^1$A″ state at the various geometries of $H_2O$ used to construct the ground- and excited-state potentials considered in the present study.

[c] Errors, in millihartree, characterizing the EOMCC($P$) energies relative to the corresponding EOMCCSDT data, which are −75.702504, −75.851860, −75.886181, −75.901368, −75.929326, −75.956186, −75.975300, −75.987453, −75.994949, −75.997508, and −75.999498 hartree for $R_{OH}$ = 1.3, 1.6, 1.809, 2.0, 2.4, 2.8, 3.2, 3.6, 4.0, 4.2, and 4.4, respectively.

[d] Errors, in millihartree, in the CC($P$;$Q$) energies relative to the corresponding EOMCCSDT data given in footnote ‘c’.

[e] The equilibrium value of the O–H bond length in the ground electronic state of water, as obtained in Ref. [S1] using the CCSD/cc-pVTZ method.

**Table S3**

Same as Table S2 for the 1 $^3$A′ state.

| $R_{OH}$ | $N_{det(in)} = 1$[a] | | $N_{det(in)} = 1,000$ | | $N_{det(in)} = 5,000$ | | $N_{det(in)} = 10,000$ | | $N_{det(in)} = 20,000$ | |
|---|---|---|---|---|---|---|---|---|---|---|
| | %T=0.0[b] | | %T=0.0–0.6[b] | | %T=3.1–9.3[b] | | %T=8.1–15.6[b] | | %T=16.7–29.1[b] | |
| | $P$[c] | ($P$;$Q$)[d] | $P$[c] | ($P$;$Q$)[d] | $P$[c] | ($P$;$Q$)[d] | $P$[c] | ($P$;$Q$)[d] | $P$[c] | ($P$;$Q$)[d] |
| 1.3 | −0.351 | 0.884 | −0.453 | 0.788 | −0.090 | 0.408 | −0.949 | 0.233 | −1.593 | 0.244 |
| 1.6 | −0.188 | 1.024 | −0.455 | 0.830 | 0.063 | 0.401 | −1.399 | 0.494 | −0.426 | 0.196 |
| 1.809[e] | 0.185 | 1.055 | −0.144 | 0.815 | 0.627 | 0.331 | −1.899 | 0.427 | −0.667 | 0.113 |
| 2.0 | 1.118 | 1.019 | 0.895 | 0.820 | −0.291 | 0.496 | −1.222 | 0.376 | −0.371 | 0.189 |
| 2.4 | 3.596 | 1.099 | 3.596 | 1.099 | 1.001 | 0.494 | 0.660 | 0.340 | 0.292 | 0.145 |
| 2.8 | 4.501 | 1.163 | 3.790 | 1.185 | 1.740 | 0.602 | 1.263 | 0.400 | 0.485 | 0.188 |
| 3.2 | 4.653 | 1.176 | 3.975 | 1.316 | 1.425 | 0.433 | 0.564 | 0.230 | 0.314 | 0.088 |
| 3.6 | 4.488 | 1.208 | 3.556 | 1.263 | 1.876 | 0.558 | 0.978 | 0.357 | 0.478 | 0.145 |
| 4.0 | 4.166 | 1.263 | 3.234 | 1.333 | 1.987 | 0.638 | 0.935 | 0.405 | 0.455 | 0.193 |
| 4.2 | 3.977 | 1.294 | 3.042 | 1.372 | 1.634 | 0.706 | 0.914 | 0.447 | 0.432 | 0.223 |
| 4.4 | 3.783 | 1.326 | 2.826 | 1.405 | 0.893 | 0.477 | 0.877 | 0.470 | 0.333 | 0.216 |

[a] The EOMCC($P$) and CC($P$;$Q$) results for the 1 $^3$A′ state at $N_{det(in)} = 1$ are equivalent to those obtained with EOMCCSD and CR-EOMCC(2,3), respectively.

[b] The %T for a given $N_{det(in)}$ is the percentage ($N_{det(in)} = 1$) or the range of percentages ($N_{det(in)} = 1,000$–$20,000$) of the $S_z = 0$ triply excited determinants captured by the CIPSI runs for the X $^1$A′ ground state at the various geometries of $H_2O$ used to construct the ground- and excited-state potentials considered in the present study.

[c] Errors, in millihartree, characterizing the EOMCC($P$) energies relative to the corresponding EOMCCSDT data, which are −75.650784, −75.793914, −75.825513, −75.842928, −75.891420, −75.937554, −75.967653, −75.985183, −75.994978, −75.998050, and −76.000308 hartree for $R_{OH}$ = 1.3, 1.6, 1.809, 2.0, 2.4, 2.8, 3.2, 3.6, 4.0, 4.2, and 4.4, respectively.

[d] Errors, in millihartree, in the CC($P$;$Q$) energies relative to the corresponding EOMCCSDT data given in footnote ‘c’.

[e] The equilibrium value of the O–H bond length in the ground electronic state of water, as obtained in Ref. [S1] using the CCSD/cc-pVTZ method.

**Table S4**
Same as Table S2 for the 1 $^3$A″ state.

| $R_{OH}$ | $N_{det(in)} = 1$[a] | | $N_{det(in)} = 1,000$ | | $N_{det(in)} = 5,000$ | | $N_{det(in)} = 10,000$ | | $N_{det(in)} = 20,000$ | |
|---|---|---|---|---|---|---|---|---|---|---|
| | %T=0.0[b] | | %T=2.2–4.3[b] | | %T=9.7–15.9[b] | | %T=13.7–23.7[b] | | %T=19.5–34.7[b] | |
| | $P$[c] | $(P;Q)$[d] | $P$[c] | $(P;Q)$[d] | $P$[c] | $(P;Q)$[d] | $P$[c] | $(P;Q)$[d] | $P$[c] | $(P;Q)$[d] |
| 1.3 | −0.325 | 0.887 | 2.295 | 1.052 | 1.362 | 0.747 | 0.902 | 0.427 | 0.391 | 0.259 |
| 1.6 | −0.205 | 1.088 | 2.897 | 1.065 | 1.392 | 0.671 | 0.833 | 0.469 | 0.422 | 0.267 |
| 1.809[e] | 0.046 | 1.110 | −0.132 | 1.010 | −0.677 | 0.643 | −1.077 | 0.314 | −1.295 | 0.116 |
| 2.0 | 0.757 | 0.999 | 3.131 | 1.172 | 1.457 | 0.708 | 0.863 | 0.535 | 0.431 | 0.295 |
| 2.4 | 3.847 | 0.663 | 2.993 | 0.688 | 1.553 | 0.705 | 0.820 | 0.420 | 0.343 | 0.205 |
| 2.8 | 7.203 | 0.326 | 3.202 | 0.640 | 1.700 | 0.753 | 0.921 | 0.507 | 0.434 | 0.230 |
| 3.2 | 10.310 | −0.212 | 4.227 | 0.652 | 1.359 | 0.609 | 0.709 | 0.331 | 0.313 | 0.151 |
| 3.6 | 13.094 | −0.899 | 3.535 | 0.836 | 1.492 | 0.720 | 1.057 | 0.493 | 0.478 | 0.301 |
| 4.0 | 15.388 | −1.594 | 3.089 | 0.888 | 1.372 | 0.749 | 0.832 | 0.518 | 0.496 | 0.340 |
| 4.2 | 16.323 | −1.909 | 4.465 | 0.978 | 1.137 | 0.611 | 0.790 | 0.527 | 0.374 | 0.235 |
| 4.4 | 17.120 | −2.192 | 4.835 | 1.010 | 0.998 | 0.416 | 0.688 | 0.399 | 0.345 | 0.203 |

[a] The EOMCC($P$) and CC($P$;$Q$) results for the 1 $^3$A″ state at $N_{det(in)} = 1$ are equivalent to those obtained with EOMCCSD and CR-EOMCC(2,3), respectively.

[b] The %T for a given $N_{det(in)}$ is the percentage ($N_{det(in)} = 1$) or the range of percentages ($N_{det(in)} = 1,000$–$20,000$) of the $S_z = 0$ triply excited determinants captured by the CIPSI runs for the 1 $^1$A″ state at the various geometries of $H_2O$ used to construct the ground- and excited-state potentials considered in the present study.

[c] Errors, in millihartree, characterizing the EOMCC($P$) energies relative to the corresponding EOMCCSDT data, which are −75.722266, −75.872393, −75.907714, −75.923946, −75.951300, −75.973528, −75.987281, −75.995001, −75.999363, −76.000790, and −76.001888 hartree for $R_{OH}$ = 1.3, 1.6, 1.809, 2.0, 2.4, 2.8, 3.2, 3.6, 4.0, 4.2, and 4.4, respectively.

[d] Errors, in millihartree, in the CC($P$;$Q$) energies relative to the corresponding EOMCCSDT data given in footnote ‘c’.

[e] The equilibrium value of the O–H bond length in the ground electronic state of water, as obtained in Ref. [S1] using the CCSD/cc-pVTZ method.

**Table S5**
Same as Table S2 for the 1 $^1$A′ state.

| $R_{OH}$ | $N_{det(in)} = 1$[a] | | $N_{det(in)} = 1,000$ | | $N_{det(in)} = 5,000$ | | $N_{det(in)} = 10,000$ | | $N_{det(in)} = 20,000$ | |
|---|---|---|---|---|---|---|---|---|---|---|
| | %T=0.0[b] | | %T=0.0–0.6[b] | | %T=3.1–9.3[b] | | %T=8.1–15.6[b] | | %T=16.7–29.1[b] | |
| | $P$[c] | $(P;Q)$[d] | $P$[c] | $(P;Q)$[d] | $P$[c] | $(P;Q)$[d] | $P$[c] | $(P;Q)$[d] | $P$[c] | $(P;Q)$[d] |
| 1.3 | −0.018 | 0.964 | −0.109 | 0.861 | 0.210 | 0.459 | −0.694 | 0.269 | −1.408 | 0.302 |
| 1.6 | 0.298 | 1.129 | −0.008 | 0.933 | 0.350 | 0.450 | −1.210 | 0.551 | −0.222 | 0.217 |
| 1.809[e] | 0.890 | 1.189 | 0.592 | 0.953 | 1.060 | 0.399 | −1.582 | 0.477 | −0.623 | 0.125 |
| 2.0 | 1.950 | 1.147 | 1.757 | 0.953 | 0.111 | 0.568 | −0.653 | 0.454 | −0.036 | 0.191 |
| 2.4 | 5.922 | 0.781 | 5.922 | 0.781 | 3.314 | 0.607 | 2.654 | 0.428 | 1.339 | 0.144 |
| 2.8 | 10.351 | 0.088 | 8.103 | 0.712 | 7.087 | 0.865 | 5.870 | 0.584 | 3.460 | 0.379 |
| 3.2 | 14.047 | −0.790 | 13.081 | 0.497 | 8.221 | 0.706 | 7.134 | 0.293 | 5.031 | 0.203 |
| 3.6 | 17.027 | −1.737 | 16.155 | 0.766 | 12.640 | 0.718 | 9.758 | 0.576 | 5.283 | 0.147 |
| 4.0 | 19.348 | −2.649 | 18.895 | 0.592 | 17.414 | 0.472 | 8.985 | 0.326 | 6.708 | −0.015 |
| 4.2 | 20.261 | −3.063 | 19.940 | 0.511 | 17.779 | 0.340 | 9.130 | 0.167 | 6.852 | −0.031 |
| 4.4 | 21.024 | −3.448 | 21.024 | 0.451 | 9.362 | 0.076 | 9.351 | 0.071 | 7.095 | −0.108 |

[a] The EOMCC($P$) and CC($P$;$Q$) results for the 1 $^1$A′ state at $N_{det(in)} = 1$ are equivalent to those obtained with EOMCCSD and CR-EOMCC(2,3), respectively.

[b] The %T for a given $N_{det(in)}$ is the percentage ($N_{det(in)} = 1$) or the range of percentages ($N_{det(in)} = 1,000$–$20,000$) of the $S_z = 0$ triply excited determinants captured by the CIPSI runs for the X $^1$A′ ground state at the various geometries of $H_2O$ used to construct the ground- and excited-state potentials considered in the present study.

[c] Errors, in millihartree, characterizing the EOMCC($P$) energies relative to the corresponding EOMCCSDT data, which are −75.628899, −75.771190, −75.799146, −75.806139, −75.810399, −75.818515, −75.827420, −75.834787, −75.840275, −75.842366, and −75.844081 hartree for $R_{OH}$ = 1.3, 1.6, 1.809, 2.0, 2.4, 2.8, 3.2, 3.6, 4.0, 4.2, and 4.4, respectively.

[d] Errors, in millihartree, in the CC($P$;$Q$) energies relative to the corresponding EOMCCSDT data given in footnote ‘c’.

[e] The equilibrium value of the O–H bond length in the ground electronic state of water, as obtained in Ref. [S1] using the CCSD/cc-pVTZ method.

**Table S6**
Same as Table S2 for the $2\,^3A'$ state.

| $R_{OH}$ | $N_{det(in)} = 1$[a] | | $N_{det(in)} = 1,000$ | | $N_{det(in)} = 5,000$ | | $N_{det(in)} = 10,000$ | | $N_{det(in)} = 20,000$ | |
|---|---|---|---|---|---|---|---|---|---|---|
| | %T=0.0[b] | | %T=0.0–0.6[b] | | %T=3.1–9.3[b] | | %T=8.1–15.6[b] | | %T=16.7–29.1[b] | |
| | $P$[c] | $(P;Q)$[d] | $P$[c] | $(P;Q)$[d] | $P$[c] | $(P;Q)$[d] | $P$[c] | $(P;Q)$[d] | $P$[c] | $(P;Q)$[d] |
| 1.3 | −0.930 | 0.877 | −1.013 | 0.776 | −1.677 | 0.492 | −0.871 | 0.197 | −1.514 | 0.187 |
| 1.6 | −0.057 | 0.950 | −0.254 | 0.797 | −0.789 | 0.417 | −0.939 | 0.257 | −1.164 | 0.154 |
| 1.809[e] | 0.958 | 1.006 | 0.709 | 0.816 | 0.264 | 0.504 | −0.117 | 0.192 | −0.320 | 0.014 |
| 2.0 | 1.668 | 1.122 | 1.515 | 0.972 | 0.868 | 0.547 | 0.573 | 0.346 | 0.213 | 0.151 |
| 2.4 | 4.621 | 0.995 | 4.621 | 0.995 | 3.363 | 0.563 | 1.929 | 0.427 | 0.973 | 0.166 |
| 2.8 | 8.219 | 0.352 | 7.427 | 0.767 | 5.927 | 0.786 | 4.782 | 0.565 | 2.317 | 0.318 |
| 3.2 | 11.562 | −0.328 | 11.182 | 0.596 | 6.775 | 0.638 | 5.615 | 0.220 | 3.984 | 0.170 |
| 3.6 | 14.620 | −1.109 | 13.799 | 0.803 | 10.767 | 0.642 | 8.054 | 0.511 | 4.590 | 0.137 |
| 4.0 | 17.204 | −1.892 | 16.374 | 0.631 | 15.145 | 0.348 | 7.992 | 0.332 | 6.128 | 0.009 |
| 4.2 | 18.274 | −2.253 | 17.504 | 0.563 | 15.331 | 0.219 | 8.215 | 0.197 | 6.439 | −0.017 |
| 4.4 | 19.197 | −2.590 | 18.144 | 0.465 | 8.511 | 0.108 | 8.497 | 0.102 | 6.694 | −0.081 |

[a] The EOMCC($P$) and CC($P$;$Q$) results for the $2\,^3A'$ state at $N_{det(in)} = 1$ are equivalent to those obtained with EOMCCSD and CR-EOMCC(2,3), respectively.
[b] The %T for a given $N_{det(in)}$ is the percentage ($N_{det(in)} = 1$) or the range of percentages ($N_{det(in)} = 1,000$–$20,000$) of the $S_z = 0$ triply excited determinants captured by the CIPSI runs for the X $^1A'$ ground state at the various geometries of $H_2O$ used to construct the ground- and excited-state potentials considered in the present study.
[c] Errors, in millihartree, characterizing the EOMCC($P$) energies relative to the corresponding EOMCCSDT data, which are −75.556467, −75.709251, −75.748568, −75.762832, −75.785421, −75.815525, −75.831462, −75.839577, −75.843920, −75.845298, and −75.846350 hartree for $R_{OH}$ = 1.3, 1.6, 1.809, 2.0, 2.4, 2.8, 3.2, 3.6, 4.0, 4.2, and 4.4, respectively.
[d] Errors, in millihartree, in the CC($P$;$Q$) energies relative to the corresponding EOMCCSDT data given in footnote ‘c’.
[e] The equilibrium value of the O–H bond length in the ground electronic state of water, as obtained in Ref. [S1] using the CCSD/cc-pVTZ method.

**Table S7**
Same as Table S2 for the $2\,^3A''$ state.

| $R_{OH}$ | $N_{det(in)} = 1$[a] | | $N_{det(in)} = 1,000$ | | $N_{det(in)} = 5,000$ | | $N_{det(in)} = 10,000$ | | $N_{det(in)} = 20,000$ | |
|---|---|---|---|---|---|---|---|---|---|---|
| | %T=0.0[b] | | %T=2.2–4.3[b] | | %T=9.7–15.9[b] | | %T=13.7–23.7[b] | | %T=19.5–34.7[b] | |
| | $P$[c] | $(P;Q)$[d] | $P$[c] | $(P;Q)$[d] | $P$[c] | $(P;Q)$[d] | $P$[c] | $(P;Q)$[d] | $P$[c] | $(P;Q)$[d] |
| 1.3 | −0.547 | 0.933 | −0.529 | 0.931 | 3.028 | 0.553 | 2.724 | 0.178 | 2.345 | 0.198 |
| 1.6 | 0.285 | 1.044 | −0.003 | 0.913 | −0.043 | 0.617 | 3.120 | 0.177 | 2.698 | 0.099 |
| 1.809[e] | 1.181 | 1.049 | 2.962 | 0.976 | 1.144 | 0.681 | 0.460 | 0.346 | 0.116 | 0.139 |
| 2.0 | 1.877 | 1.052 | 1.656 | 0.980 | 2.514 | 0.569 | 3.582 | 0.323 | 1.231 | 0.313 |
| 2.4 | 2.210 | 1.111 | 2.300 | 1.147 | 3.093 | 0.813 | 1.192 | 0.481 | 0.655 | 0.262 |
| 2.8 | 2.703 | 1.472 | 5.725 | 1.916 | 4.161 | 0.701 | 1.748 | 0.598 | 1.070 | 0.267 |
| 3.2 | 5.070 | 2.801 | 8.721 | 2.870 | 6.058 | 0.811 | 3.342 | 0.584 | 0.893 | 0.132 |
| 3.6 | 11.868 | 6.745 | 11.498 | 3.277 | 5.922 | 0.599 | 5.360 | 0.468 | 1.299 | 0.223 |
| 4.0 | 21.864 | 11.890 | 13.281 | 3.471 | 6.357 | 0.605 | 4.226 | 0.300 | 2.256 | 0.174 |
| 4.2 | 25.767 | 13.294 | 22.294 | 5.768 | 6.052 | 0.587 | 3.961 | 0.308 | 2.051 | 0.177 |
| 4.4 | 28.470 | 13.976 | 23.874 | 5.789 | 7.544 | 1.112 | 4.298 | 0.374 | 2.704 | 0.209 |

[a] The EOMCC($P$) and CC($P$;$Q$) results for the $2\,^3A''$ state at $N_{det(in)} = 1$ are equivalent to those obtained with EOMCCSD and CR-EOMCC(2,3), respectively.
[b] The %T for a given $N_{det(in)}$ is the percentage ($N_{det(in)} = 1$) or the range of percentages ($N_{det(in)} = 1,000$–$20,000$) of the $S_z = 0$ triply excited determinants captured by the CIPSI runs for the $1\,^1A''$ state at the various geometries of $H_2O$ used to construct the ground- and excited-state potentials considered in the present study.
[c] Errors, in millihartree, characterizing the EOMCC($P$) energies relative to the corresponding EOMCCSDT data, which are −75.624198, −75.781036, −75.821469, −75.835975, −75.828038, −75.801866, −75.778512, −75.765773, −75.763214, −75.762712, and −75.761785 hartree for $R_{OH}$ = 1.3, 1.6, 1.809, 2.0, 2.4, 2.8, 3.2, 3.6, 4.0, 4.2, and 4.4, respectively.
[d] Errors, in millihartree, in the CC($P$;$Q$) energies relative to the corresponding EOMCCSDT data given in footnote ‘c’.
[e] The equilibrium value of the O–H bond length in the ground electronic state of water, as obtained in Ref. [S1] using the CCSD/cc-pVTZ method.

**Table S8**
Same as Table S2 for the 2 $^1$A′ state.

| $R_{OH}$ | $N_{det(in)}$ = 1[a] | | $N_{det(in)}$ = 1,000 | | $N_{det(in)}$ = 5,000 | | $N_{det(in)}$ = 10,000 | | $N_{det(in)}$ = 20,000 | |
|---|---|---|---|---|---|---|---|---|---|---|
| | %T=0.0[b] | | %T=0.0–0.6[b] | | %T=3.1–9.3[b] | | %T=8.1–15.6[b] | | %T=16.7–29.1[b] | |
| | $P$[c] | $(P;Q)$[d] | $P$[c] | $(P;Q)$[d] | $P$[c] | $(P;Q)$[d] | $P$[c] | $(P;Q)$[d] | $P$[c] | $(P;Q)$[d] |
| 1.3 | −0.720 | 0.865 | −0.804 | 0.762 | −1.485 | 0.490 | −0.682 | 0.209 | −1.315 | 0.226 |
| 1.6 | 0.014 | 0.918 | −0.187 | 0.759 | −0.681 | 0.431 | −0.764 | 0.303 | −0.842 | 0.244 |
| 1.809[e] | 0.920 | 0.908 | 0.665 | 0.713 | 0.274 | 0.466 | −0.030 | 0.228 | −0.226 | 0.053 |
| 2.0 | 1.886 | 0.872 | 1.730 | 0.715 | 1.228 | 0.441 | 1.076 | 0.350 | 0.915 | 0.210 |
| 2.4 | 5.132 | 1.267 | 5.132 | 1.267 | 3.125 | 0.933 | 2.714 | 0.481 | 1.420 | 0.298 |
| 2.8 | 11.838 | 0.215 | 10.023 | 0.461 | 5.431 | 0.920 | 3.802 | 0.603 | 2.506 | 0.256 |
| 3.2 | 18.528 | −2.178 | 14.620 | −1.306 | 7.163 | 0.279 | 4.723 | 0.306 | 1.263 | 0.205 |
| 3.6 | 25.315 | −4.968 | 12.469 | −0.298 | 9.497 | 0.348 | 8.498 | 0.440 | 3.675 | 0.696 |
| 4.0 | 30.370 | −6.883 | 10.559 | 0.517 | 6.788 | 0.938 | 5.730 | 0.745 | 2.152 | 0.463 |
| 4.2 | 31.800 | −7.063 | 10.481 | 0.744 | 5.340 | 0.732 | 2.919 | 0.594 | 1.950 | 0.289 |
| 4.4 | 32.540 | −6.732 | 32.540 | 0.859 | 2.812 | 0.404 | 2.792 | 0.396 | 1.904 | 0.187 |

[a] The EOMCC($P$) and CC($P$;$Q$) results for the 2 $^1$A′ state at $N_{det(in)}$ = 1 are equivalent to those obtained with EOMCCSD and CR-EOMCC(2,3), respectively.
[b] The %T for a given $N_{det(in)}$ is the percentage ($N_{det(in)}$ = 1) or the range of percentages ($N_{det(in)}$ = 1,000–20,000) of the $S_z$ = 0 triply excited determinants captured by the CIPSI runs for the X $^1$A′ ground state at the various geometries of $H_2O$ used to construct the ground- and excited-state potentials considered in the present study.
[c] Errors, in millihartree, characterizing the EOMCC($P$) energies relative to the corresponding EOMCCSDT data, which are −75.542618, −75.687943, −75.718367, −75.724899, −75.716154, −75.724539, −75.730092, −75.730473, −75.727678, −75.725296, and −75.722336 hartree for $R_{OH}$ = 1.3, 1.6, 1.809, 2.0, 2.4, 2.8, 3.2, 3.6, 4.0, 4.2, and 4.4, respectively.
[d] Errors, in millihartree, in the CC($P$;$Q$) energies relative to the corresponding EOMCCSDT data given in footnote ‘c’.
[e] The equilibrium value of the O–H bond length in the ground electronic state of water, as obtained in Ref. [S1] using the CCSD/cc-pVTZ method.

**Table S9**
Same as Table S2 for the 2 $^1$A″ state.

| $R_{OH}$ | $N_{det(in)}$ = 1[a] | | $N_{det(in)}$ = 1,000 | | $N_{det(in)}$ = 5,000 | | $N_{det(in)}$ = 10,000 | | $N_{det(in)}$ = 20,000 | |
|---|---|---|---|---|---|---|---|---|---|---|
| | %T=0.0[b] | | %T=2.2–4.3[b] | | %T=9.7–15.9[b] | | %T=13.7–23.7[b] | | %T=19.5–34.7[b] | |
| | $P$[c] | $(P;Q)$[d] | $P$[c] | $(P;Q)$[d] | $P$[c] | $(P;Q)$[d] | $P$[c] | $(P;Q)$[d] | $P$[c] | $(P;Q)$[d] |
| 1.3 | −0.688 | 0.912 | −0.688 | 0.920 | 3.165 | 0.580 | 2.875 | 0.203 | 2.390 | 0.207 |
| 1.6 | −0.078 | 0.963 | −0.335 | 0.850 | −0.113 | 0.643 | 3.352 | 0.234 | 2.746 | 0.093 |
| 1.809[e] | 0.649 | 0.905 | 2.842 | 0.862 | 1.347 | 0.710 | 0.686 | 0.378 | 0.331 | 0.162 |
| 2.0 | 1.251 | 0.845 | 1.122 | 0.838 | 2.492 | 0.584 | 3.606 | 0.303 | 1.235 | 0.327 |
| 2.4 | 1.371 | 0.776 | 1.678 | 0.906 | 2.975 | 0.734 | 1.068 | 0.456 | 0.611 | 0.269 |
| 2.8 | 1.147 | 0.846 | 4.767 | 1.531 | 3.963 | 0.605 | 1.534 | 0.535 | 0.992 | 0.243 |
| 3.2 | 1.309 | 1.103 | 6.120 | 1.844 | 5.044 | 0.648 | 2.388 | 0.443 | 0.808 | 0.128 |
| 3.6 | 2.177 | 1.642 | 6.150 | 1.573 | 5.261 | 0.524 | 4.986 | 0.471 | 1.237 | 0.288 |
| 4.0 | 4.156 | 2.805 | 7.117 | 2.043 | 4.944 | 0.351 | 4.415 | 0.174 | 2.222 | 0.088 |
| 4.2 | 5.598 | 3.693 | 11.962 | 3.156 | 5.295 | 0.345 | 4.440 | 0.130 | 2.197 | 0.047 |
| 4.4 | 7.284 | 4.759 | 13.405 | 3.652 | 5.282 | 0.726 | 4.706 | 0.137 | 3.175 | 0.061 |

[a] The EOMCC($P$) and CC($P$;$Q$) results for the 2 $^1$A″ state at $N_{det(in)}$ = 1 are equivalent to those obtained with EOMCCSD and CR-EOMCC(2,3), respectively.
[b] The %T for a given $N_{det(in)}$ is the percentage ($N_{det(in)}$ = 1) or the range of percentages ($N_{det(in)}$ = 1,000–20,000) of the $S_z$ = 0 triply excited determinants captured by the CIPSI runs for the 1 $^1$A″ state at the various geometries of $H_2O$ used to construct the ground- and excited-state potentials considered in the present study.
[c] Errors, in millihartree, characterizing the EOMCC($P$) energies relative to the corresponding EOMCCSDT data, which are −75.614700, −75.769204, −75.807409, −75.820292, −75.810444, −75.782217, −75.754820, −75.733362, −75.719183, −75.714539, and −75.711300 hartree for $R_{OH}$ = 1.3, 1.6, 1.809, 2.0, 2.4, 2.8, 3.2, 3.6, 4.0, 4.2, and 4.4, respectively.
[d] Errors, in millihartree, in the CC($P$;$Q$) energies relative to the corresponding EOMCCSDT data given in footnote ‘c’.
[e] The equilibrium value of the O–H bond length in the ground electronic state of water, as obtained in Ref. [S1] using the CCSD/cc-pVTZ method.

**Table S10**
Same as Table S2 for the 3 $^3$A″ state.

| $R_{OH}$ | $N_{\text{det(in)}} = 1$[a] | | $N_{\text{det(in)}} = 1,000$ | | $N_{\text{det(in)}} = 5,000$ | | $N_{\text{det(in)}} = 10,000$ | | $N_{\text{det(in)}} = 20,000$ | |
|---|---|---|---|---|---|---|---|---|---|---|
| | %T=0.0[b] | | %T=2.2–4.3[b] | | %T=9.7–15.9[b] | | %T=13.7–23.7[b] | | %T=19.5–34.7[b] | |
| | $P$[c] | $(P;Q)$[d] | $P$[c] | $(P;Q)$[d] | $P$[c] | $(P;Q)$[d] | $P$[c] | $(P;Q)$[d] | $P$[c] | $(P;Q)$[d] |
| 1.3 | 0.779 | 1.263 | 1.522 | 1.226 | 2.425 | 0.809 | 1.692 | 0.451 | 0.591 | 0.270 |
| 1.6 | 1.104 | 1.518 | 1.044 | 1.382 | 4.785 | 0.563 | 1.803 | 0.531 | 1.046 | 0.270 |
| 1.809[e] | 1.241 | 1.660 | 4.103 | 1.106 | 2.466 | 0.894 | 1.274 | 0.447 | 0.672 | 0.209 |
| 2.0 | 1.399 | 1.643 | 1.508 | 1.629 | 5.131 | 0.817 | 2.126 | 0.686 | 1.488 | 0.405 |
| 2.4 | 3.843 | 2.230 | 5.198 | 2.576 | 3.501 | 1.610 | 1.579 | 0.634 | 0.798 | 0.291 |
| 2.8 | 62.012 | 36.791 | 48.513 | 16.046 | 11.838 | 1.680 | 5.743 | 0.614 | 3.176 | 0.281 |
| 3.2 | 65.442 | 6.569 | 43.274 | 8.074 | 10.280 | 0.877 | 5.932 | 0.441 | 2.243 | 0.144 |
| 3.6 | 53.786 | −0.457 | 23.250 | 4.943 | 8.865 | 1.004 | 7.918 | 0.923 | 2.101 | 0.243 |
| 4.0 | 42.844 | −4.801 | 17.965 | 4.984 | 7.701 | 1.000 | 5.007 | 0.434 | 2.556 | 0.224 |
| 4.2 | 39.743 | −5.151 | 28.244 | 5.616 | 7.228 | 0.988 | 4.766 | 0.382 | 2.346 | 0.184 |
| 4.4 | 38.464 | −4.513 | 28.566 | 6.040 | 8.753 | 2.037 | 5.247 | 0.440 | 3.335 | 0.227 |

[a] The EOMCC($P$) and CC($P$;$Q$) results for the 3 $^3$A″ state at $N_{\text{det(in)}} = 1$ are equivalent to those obtained with EOMCCSD and CR-EOMCC(2,3), respectively.
[b] The %T for a given $N_{\text{det(in)}}$ is the percentage ($N_{\text{det(in)}} = 1$) or the range of percentages ($N_{\text{det(in)}} = 1,000$–$20,000$) of the $S_z = 0$ triply excited determinants captured by the CIPSI runs for the 1 $^1$A″ state at the various geometries of $H_2O$ used to construct the ground- and excited-state potentials considered in the present study.
[c] Errors, in millihartree, characterizing the EOMCC($P$) energies relative to the corresponding EOMCCSDT data, which are −75.370374, −75.516222, −75.554100, −75.582672, −75.602051, −75.654784, −75.698187, −75.716719, −75.718451, −75.717253, and −75.716073 hartree for $R_{OH}$ = 1.3, 1.6, 1.809, 2.0, 2.4, 2.8, 3.2, 3.6, 4.0, 4.2, and 4.4, respectively.
[d] Errors, in millihartree, in the CC($P$;$Q$) energies relative to the corresponding EOMCCSDT data given in footnote 'c'.
[e] The equilibrium value of the O–H bond length in the ground electronic state of water, as obtained in Ref. [S1] using the CCSD/cc-pVTZ method.

**Table S11**
Same as Table S2 for the 3 $^1$A′ state.

| $R_{OH}$ | $N_{\text{det(in)}} = 1$[a] | | $N_{\text{det(in)}} = 1,000$ | | $N_{\text{det(in)}} = 5,000$ | | $N_{\text{det(in)}} = 10,000$ | | $N_{\text{det(in)}} = 20,000$ | |
|---|---|---|---|---|---|---|---|---|---|---|
| | %T=0.0[b] | | %T=0.0–0.6[b] | | %T=3.1–9.3[b] | | %T=8.1–15.6[b] | | %T=16.7–29.1[b] | |
| | $P$[c] | $(P;Q)$[d] | $P$[c] | $(P;Q)$[d] | $P$[c] | $(P;Q)$[d] | $P$[c] | $(P;Q)$[d] | $P$[c] | $(P;Q)$[d] |
| 1.3 | 1.189 | 1.471 | 1.070 | 1.312 | 1.428 | 0.668 | 1.142 | 0.330 | 0.252 | 0.248 |
| 1.6 | 1.674 | 1.605 | 1.226 | 1.157 | 0.700 | 0.787 | 1.416 | 0.433 | 1.554 | 0.040 |
| 1.809[e] | 2.399 | 1.598 | 2.009 | 1.240 | 1.461 | 0.810 | 1.073 | 0.483 | 0.890 | 0.321 |
| 2.0 | 3.392 | 1.517 | 3.169 | 1.267 | 2.423 | 0.764 | 2.176 | 0.628 | 1.632 | 0.352 |
| 2.4 | 5.272 | 0.714 | 5.272 | 0.714 | 2.844 | 0.546 | 1.936 | 0.233 | 0.993 | 0.075 |
| 2.8 | 6.462 | 0.852 | 5.555 | 0.852 | 4.990 | 0.812 | 3.094 | 0.604 | 1.779 | 0.393 |
| 3.2 | 12.832 | 2.422 | 11.708 | 2.316 | 6.203 | 1.935 | 5.652 | 1.611 | 3.456 | 1.208 |
| 3.6 | 23.485 | 5.089 | 20.022 | 4.461 | 13.850 | 4.639 | 9.973 | 4.403 | 7.191 | 4.021 |
| 4.0 | 28.958 | 4.584 | 22.945 | 5.322 | 16.183 | 5.544 | 11.734 | 5.431 | 9.336 | 5.104 |
| 4.2 | 30.434 | 3.564 | 23.117 | 5.495 | 16.045 | 5.828 | 10.678 | 3.945 | 8.950 | 3.493 |
| 4.4 | 32.035 | 2.204 | 32.035 | 5.726 | 11.113 | 3.931 | 11.094 | 3.933 | 8.920 | 3.133 |

[a] The EOMCC($P$) and CC($P$;$Q$) results for the 3 $^1$A′ state at $N_{\text{det(in)}} = 1$ are equivalent to those obtained with EOMCCSD and CR-EOMCC(2,3), respectively.
[b] The %T for a given $N_{\text{det(in)}}$ is the percentage ($N_{\text{det(in)}} = 1$) or the range of percentages ($N_{\text{det(in)}} = 1,000$–$20,000$) of the $S_z = 0$ triply excited determinants captured by the CIPSI runs for the X $^1$A′ ground state at the various geometries of $H_2O$ used to construct the ground- and excited-state potentials considered in the present study.
[c] Errors, in millihartree, characterizing the EOMCC($P$) energies relative to the corresponding EOMCCSDT data, which are −75.391520, −75.578996, −75.637243, −75.668055, −75.696531, −75.678272, −75.661466, −75.660620, −75.665098, −75.665657, and −75.664958 hartree for $R_{OH}$ = 1.3, 1.6, 1.809, 2.0, 2.4, 2.8, 3.2, 3.6, 4.0, 4.2, and 4.4, respectively.
[d] Errors, in millihartree, in the CC($P$;$Q$) energies relative to the corresponding EOMCCSDT data given in footnote 'c'.
[e] The equilibrium value of the O–H bond length in the ground electronic state of water, as obtained in Ref. [S1] using the CCSD/cc-pVTZ method.

**Table S12**
Same as Table S2 for the 3 $^3$A′ state.

| $R_{OH}$ | $N_{det(in)} = 1$[a] | | $N_{det(in)} = 1,000$ | | $N_{det(in)} = 5,000$ | | $N_{det(in)} = 10,000$ | | $N_{det(in)} = 20,000$ | |
|---|---|---|---|---|---|---|---|---|---|---|
| | %T=0.0[b] | | %T=0.0–0.6[b] | | %T=3.1–9.3[b] | | %T=8.1–15.6[b] | | %T=16.7–29.1[b] | |
| | $P$[c] | $(P;Q)$[d] | $P$[c] | $(P;Q)$[d] | $P$[c] | $(P;Q)$[d] | $P$[c] | $(P;Q)$[d] | $P$[c] | $(P;Q)$[d] |
| 1.3 | 0.720 | 1.272 | 0.599 | 1.119 | 0.814 | 0.544 | 0.502 | 0.248 | −0.229 | 0.164 |
| 1.6 | 1.352 | 1.531 | 0.935 | 1.107 | 0.292 | 0.691 | 0.877 | 0.368 | 1.246 | 0.050 |
| 1.809[e] | 2.074 | 1.592 | 1.704 | 1.261 | 1.100 | 0.778 | 0.706 | 0.451 | 0.511 | 0.282 |
| 2.0 | 2.950 | 1.393 | 2.759 | 1.172 | 1.921 | 0.670 | 1.702 | 0.539 | 1.307 | 0.341 |
| 2.4 | 3.158 | 0.986 | 3.158 | 0.986 | 1.412 | 0.745 | 1.163 | 0.256 | 0.200 | 0.135 |
| 2.8 | 4.223 | 1.175 | 3.901 | 1.050 | 3.275 | 0.942 | 1.855 | 0.676 | 0.796 | 0.400 |
| 3.2 | 6.986 | 1.528 | 6.629 | 1.433 | 1.656 | 0.960 | 3.560 | 0.869 | 1.780 | 0.447 |
| 3.6 | 11.320 | 2.330 | 9.537 | 2.270 | 5.262 | 1.701 | 2.739 | 1.274 | 0.999 | 0.909 |
| 4.0 | 16.730 | 3.829 | 14.045 | 4.522 | 12.336 | 2.489 | 6.967 | 2.709 | 5.426 | 2.461 |
| 4.2 | 19.566 | 5.000 | 15.671 | 6.323 | 14.631 | 3.148 | 7.979 | 1.904 | 6.102 | 1.789 |
| 4.4 | 22.282 | 6.656 | 16.955 | 7.603 | 9.131 | 2.265 | 9.119 | 2.264 | 6.966 | 2.106 |

[a] The EOMCC($P$) and CC($P$;$Q$) results for the 3 $^3$A′ state at $N_{det(in)} = 1$ are equivalent to those obtained with EOMCCSD and CR-EOMCC(2,3), respectively.

[b] The %T for a given $N_{det(in)}$ is the percentage ($N_{det(in)} = 1$) or the range of percentages ($N_{det(in)} = 1,000$–$20,000$) of the $S_z = 0$ triply excited determinants captured by the CIPSI runs for the X $^1$A′ ground state at the various geometries of $H_2O$ used to construct the ground- and excited-state potentials considered in the present study.

[c] Errors, in millihartree, characterizing the EOMCC($P$) energies relative to the corresponding EOMCCSDT data, which are −75.444133, −75.619787, −75.676486, −75.714899, −75.737345, −75.705526, −75.675863, −75.654127, −75.640046, −75.635295, and −75.631806 hartree for $R_{OH}$ = 1.3, 1.6, 1.809, 2.0, 2.4, 2.8, 3.2, 3.6, 4.0, 4.2, and 4.4, respectively.

[d] Errors, in millihartree, in the CC($P$;$Q$) energies relative to the corresponding EOMCCSDT data given in footnote ‘c’.

[e] The equilibrium value of the O–H bond length in the ground electronic state of water, as obtained in Ref. [S1] using the CCSD/cc-pVTZ method.
